# Supplementary material for: TellusLoom: Weaving Knowledge into Synthetic Worlds for Dense Prediction in Remote Sensing
Source: arXiv:2611.40887 source file (2026-11-30)
Supplement: Supplementary file 1 [file supp_contents.tex]

\makeatletter
\newcommand\SuppTocStart{}%
\newcommand\SuppContentsSetup{%
  \def\cvprsect##1{\cvprsection[##1]{\texorpdfstring{\hskip -1em.~}{}##1}}%
  \def\cvprsubsect##1{\cvprsubsection[##1]{\texorpdfstring{\hskip -1em.~}{}##1}}%
  \addtocontents{toc}{\protect\SuppTocStart}%
  \pdfbookmark[0]{Supplementary Material}{supp.material}}
\newcommand\printsuppcontents{%
  \section*{Supplementary contents}%
  \begingroup
    \setcounter{tocdepth}{2}%
    \renewcommand\@pnumwidth{2.2em}%
    \renewcommand\@tocrmarg{2.55em plus 1fil}%
    \hypersetup{linktoc=all}%
    \let\Supp@contentsline\contentsline
    \def\contentsline##1##2##3##4{}%
    \def\SuppTocStart{\let\contentsline\Supp@contentsline}%
    \@starttoc{toc}%
  \endgroup
  \par\medskip}%
\newcount\Supp@seccount
\newtoks\Supp@lefttoks
\newtoks\Supp@righttoks
\def\Supp@split{5}%
\def\Supp@sectionword{section}
\def\Supp@collect#1#2#3#4{%
  \def\Supp@kind{#1}%
  \ifx\Supp@kind\Supp@sectionword \global\advance\Supp@seccount by 1 \fi
  \ifnum\Supp@seccount<\Supp@split\relax
    \global\Supp@lefttoks\expandafter{\the\Supp@lefttoks\Supp@contentsline{#1}{#2}{#3}{#4}}%
  \else
    \global\Supp@righttoks\expandafter{\the\Supp@righttoks\Supp@contentsline{#1}{#2}{#3}{#4}}%
  \fi}
\newcommand\SuppTitleWithContents{%
  \newpage
  \twocolumn[{%
    \centering
    {\Large \textbf{\thetitle}\\ \vspace{0.5em}Supplementary Material\\ \vspace{1.0em}}%
    \begingroup
      \normalsize\normalfont\raggedright
      {\large\bfseries Supplementary contents\par}\vspace{6pt}%
      \setcounter{tocdepth}{2}%
      \renewcommand\@pnumwidth{2.2em}%
      \renewcommand\@tocrmarg{2.55em plus 1fil}%
      \hypersetup{linktoc=all}%
      \let\Supp@contentsline\contentsline
      \global\Supp@seccount=0 \global\Supp@lefttoks{}\global\Supp@righttoks{}%
      \def\contentsline##1##2##3##4{}%
      \def\SuppTocStart{\let\contentsline\Supp@collect}%
      \@starttoc{toc}%
      \noindent
      \begin{minipage}[t]{\columnwidth}\the\Supp@lefttoks\end{minipage}\hfill
      \begin{minipage}[t]{\columnwidth}\the\Supp@righttoks\end{minipage}\par
    \endgroup
    \vspace{16pt}%
  }]}
\makeatother
